# Supplementary material for: Exploring kinase DFG loop conformational stability with AlphaFold2-RAVE
Source: arXiv:2309.03649 ancillary file (2023-09-07)
Supplement: Supplementary file 1 [file supplement.pdf]

# Supplementary Material for "Exploring kinase DFG loop conformational stability with AlphaFold2-RAVE"

Bodhi P. Vani,[†] Akashnathan Aranganathan,[‡] and Pratyush Tiwary[*,¶,§]

†*Institute for Physical Science and Technology, University of Maryland, College Park, Maryland 20742, USA*

‡*Biophysics Program and Institute for Physical Science and Technology, University of Maryland, College Park 20742, USA*

¶*Department of Chemistry and Biochemistry and Institute for Physical Science and Technology, University of Maryland, College Park 20742, USA*

§*Corresponding author*

E-mail: ptiwary@umd.edu

## Collective variables

Collective variables described in the main text are defined in detail in tables **??**, and visually represented in 1. Distributions obtained from reduced MSA AF2 are shown in Fig. 2.

## Comparison of AF2 results across kinases

In Fig3, we show structural diversity obtained from reduced MSA AF2 for two other kinases in comparison with DDR1, specifically the Abl and Src kinases. We specifically choose

Table 1: Residues included in collective variable definitions

| **Universal kinase motif** | **Conserved residue** | **ID for DDR1** | **Description** |
|---|---|---|---|
| HRDxN | Asn | 173 | Asn of the HRDxxxxN motif |
| DFGAsp | Asp | 186 | Asp of DFG motif |
| DFGPhe | Phe | 187 | Phe of DFG motif |
| DFGGly | Gly | 188 | Gly of DFG motif |
| ChelE | Glu | 74 | C-helix conserved Glu |
| ChelX | - | 78 | Four down from the C-helix conserved Glu |
| X2 | - | 81 | C-terminal of C-alpha helix |
| X3 | - | 165 | Midpoint of section in Clobe roughly parallel to DFG motif |
| X4 | - | 189 | Three down from DFG |
| sbridgeR | Arg | 172 | Conserved Arginine that makes a salt bridge with C-helix Glu |
| sbridgeK | Lys | 57 | Conserved Lysine that makes a salt bridge with C-helix Glu |
| PloopN1 | - | 18 | First residue of the P-loop |
| PloopC1 | - | 23 | Last residue of the P-loop |

Table 2: Distances used as input collective variables for SPIB

| **Distances** | | | |
|---|---|---|---|
| **Kinase motif** | **Atom name** | **Kinase motif** | **Atom name** |
| HRDxN | CA | DFGPhe | CA |
| ChelE | CA | DFGPhe | CA |
| PloopN1 | CA | PloopC1 | CA |
| PloopN2 | CA | PloopC2 | CA |
| DFGAsp | CG | HRDxN | CA |
| DFGPhe | CG | X2 | CA |
| sbridgeR | CZ | ChelE | CD |
| sbridgeK | NZ | ChelE | CD |
| DFGGly | O | sbridgeR | N |
| ChelX | CA | DFGPhe | CZ |
| sbridgeK | CA | DFGPhe | CZ |
| sbridgeK | CB | ChelE | CB |
| sbridgeK | CB | DFGAsp | CB |
| X2 | CA | X4 | CA |

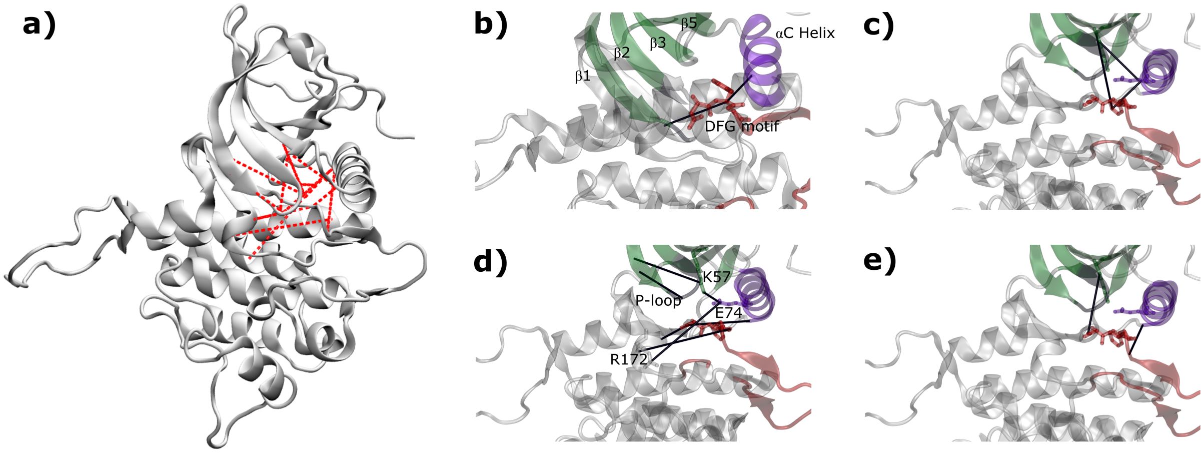


Figure 1: a) Visualization of input CVs for SPIB in red dashed lines, detailed visualization of the CVs in b)-e) in black lines. b) CVs corresponding to the A-loop distance with N lobe $\alpha$C helix and C lobe N173,[1] c) CVs used for Dunbrack classification of DFG in/inter/out conformations that primarily focus on distances between DFG Phe and the conserved salt bridge between K57 and E74 present in the N lobe,[2] d) CVs corresponding to A-loop DFG motif distances with to N lobe $\alpha$C helix and C lobe R172. These CVs also represent the dissociation of the conserved salt bridge by including the salt bridge distance, as in c), and the structural integrity of the P-loop. e) CVs corresponding to A-loop DFG motif distance with N lobe $\alpha$C helix and $\beta$3.

these kinases as they are well known to have very different stabilities for the active and inactive states, are well studied, and are of medical importance.[3] It is clear that there is very no qualitative difference and very little quantitative difference in AF2's predictions for these three kinases– suggesting that for homologous molecules, AF2 learns very limited structural information. At low MSA depths (e.g. 8), AF2 generates diverse conformations almost agnostic to specific kinase identities, while at even slightly higher MSA depths (e.g. 16), AF2 does not see statistically significant diversity in either kinase sequence, with a strong bias towards the DFG-in active conformation. A detailed analysis of the effect of the MSA length on the conformational diversity of all three kinases is presented in the SI. As suggested in Monteiro et al.,[4] varying MSA length can provide a qualitative understanding of the relative population for some sequences. Here, we see that for DFG-in dominant kinases like Abl and Src, this hypothesis is true. However, the relative populations are flipped for DFG-out dominant kinases like DDR1, and it is furthermore evident from 3 that relative

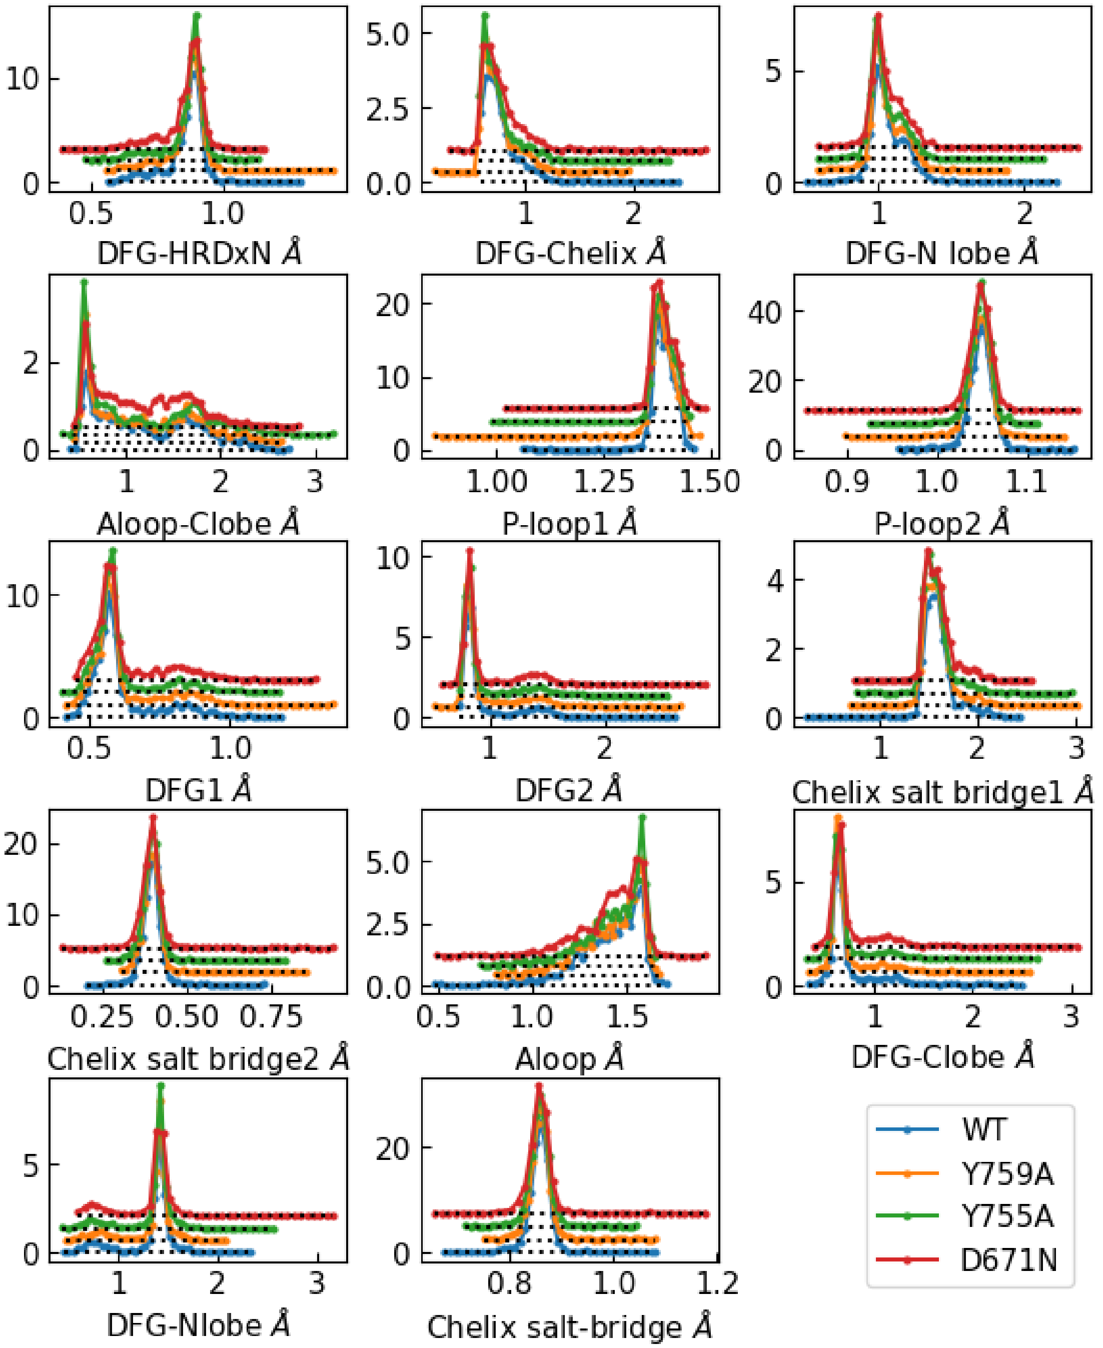


Figure 2: Collective variable distributions for reduced MSA AF2 structures for wild type and mutants D671N, Y755A, and Y759A. These CVs are described in Table 1, and represent a large number of important collective motions in the molecule. The distributions have been plotted with offsets since these are highly overlapping and similar, indicating that AF2 even with reduced MSA can not distinguish between conformational stabilities of these sequences. The zero lines are marked with dashed black lines.

populations for all kinases are uncorrelated with Boltzmann stabilities. Reweighting these populations with their corresponding Boltzmann weights is the primary motivation for this work.

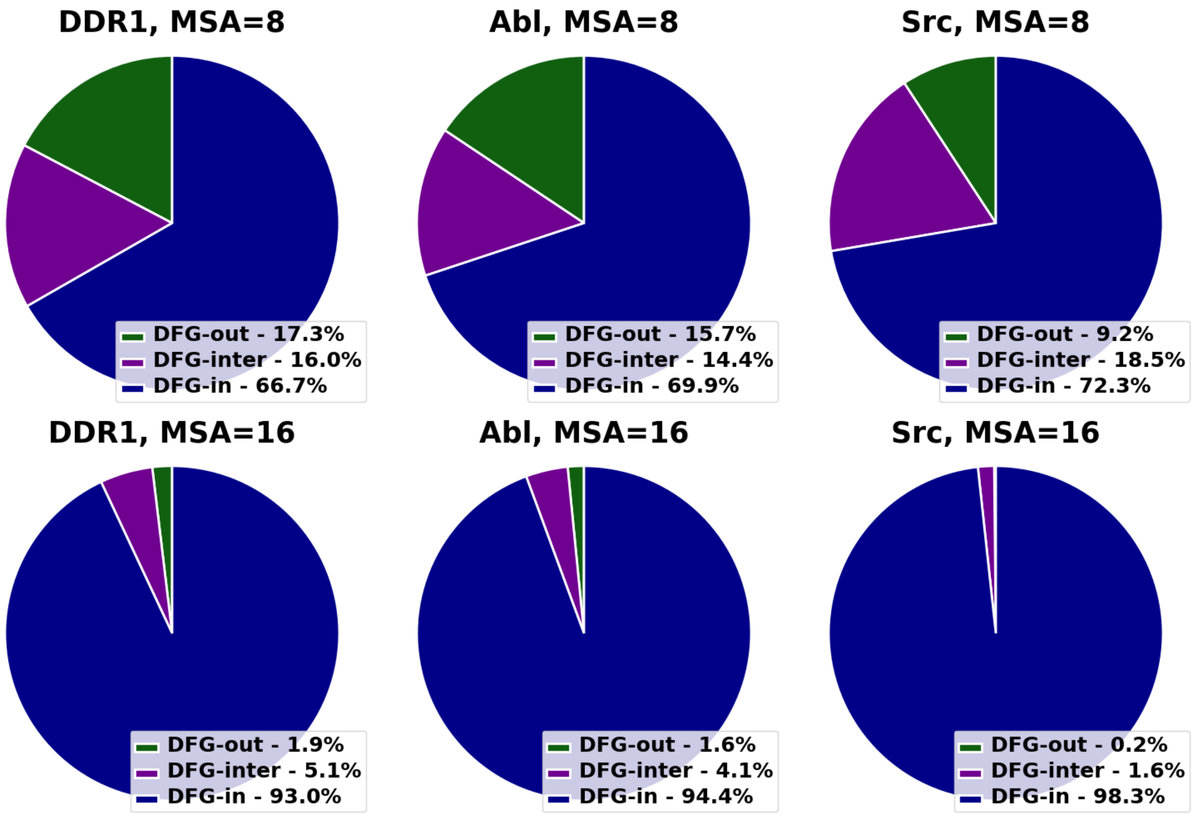


Figure 3: Statistics of structural diversity obtained from AF2 reduced MSA on three kinases: DDR1, Abl, and Src, showing that AF2 does not really distinguish between them.

# Sampling results

The bias potential learnt to perform our final calculations is shown in Fig. 4. Our final combined bias potentials are shown in Fig. 5.

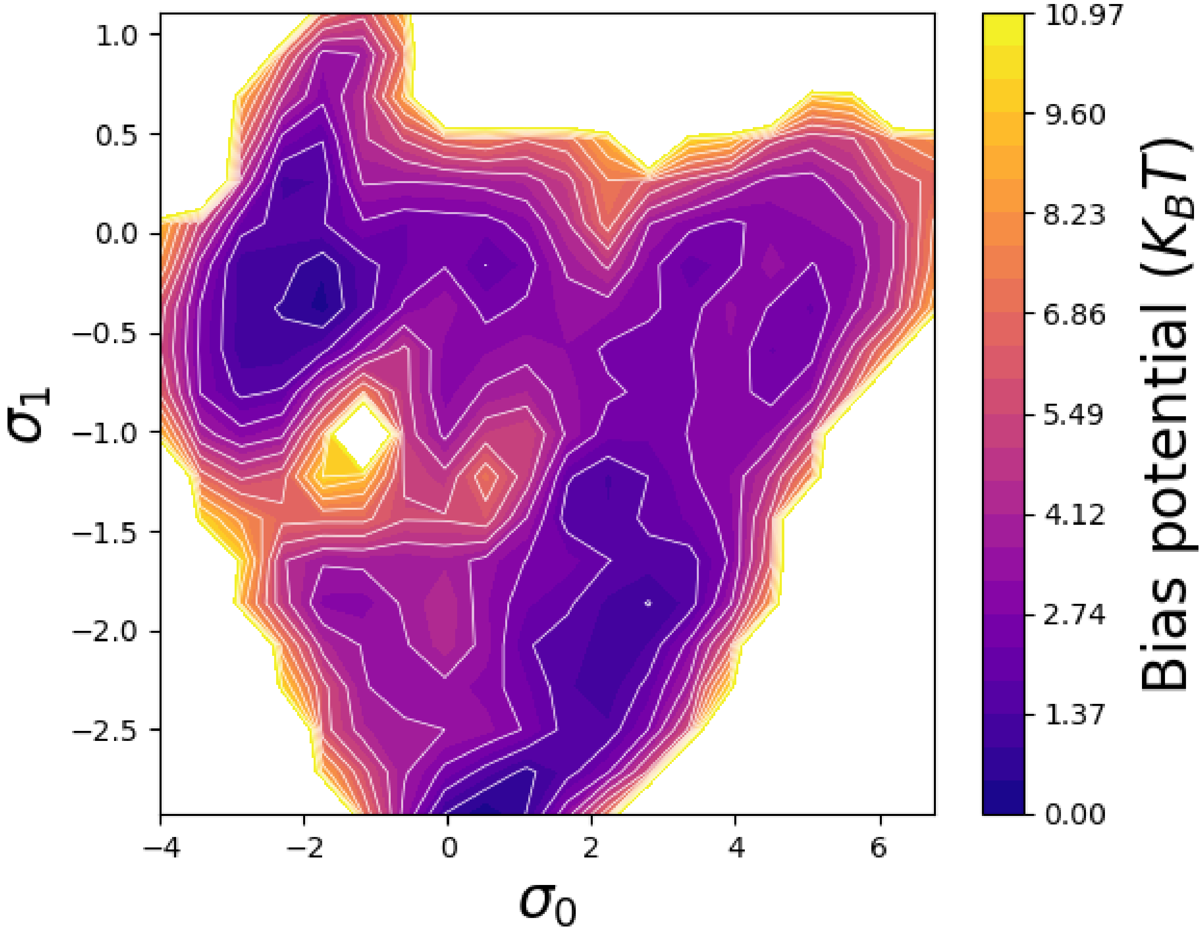


Figure 4: Bias potential learnt from metadynamics on SPIB learnt from unbiased AF2RAVE seeded trajectories. The potential is plotted on SPIB coordinates $\sigma_{0,1}$

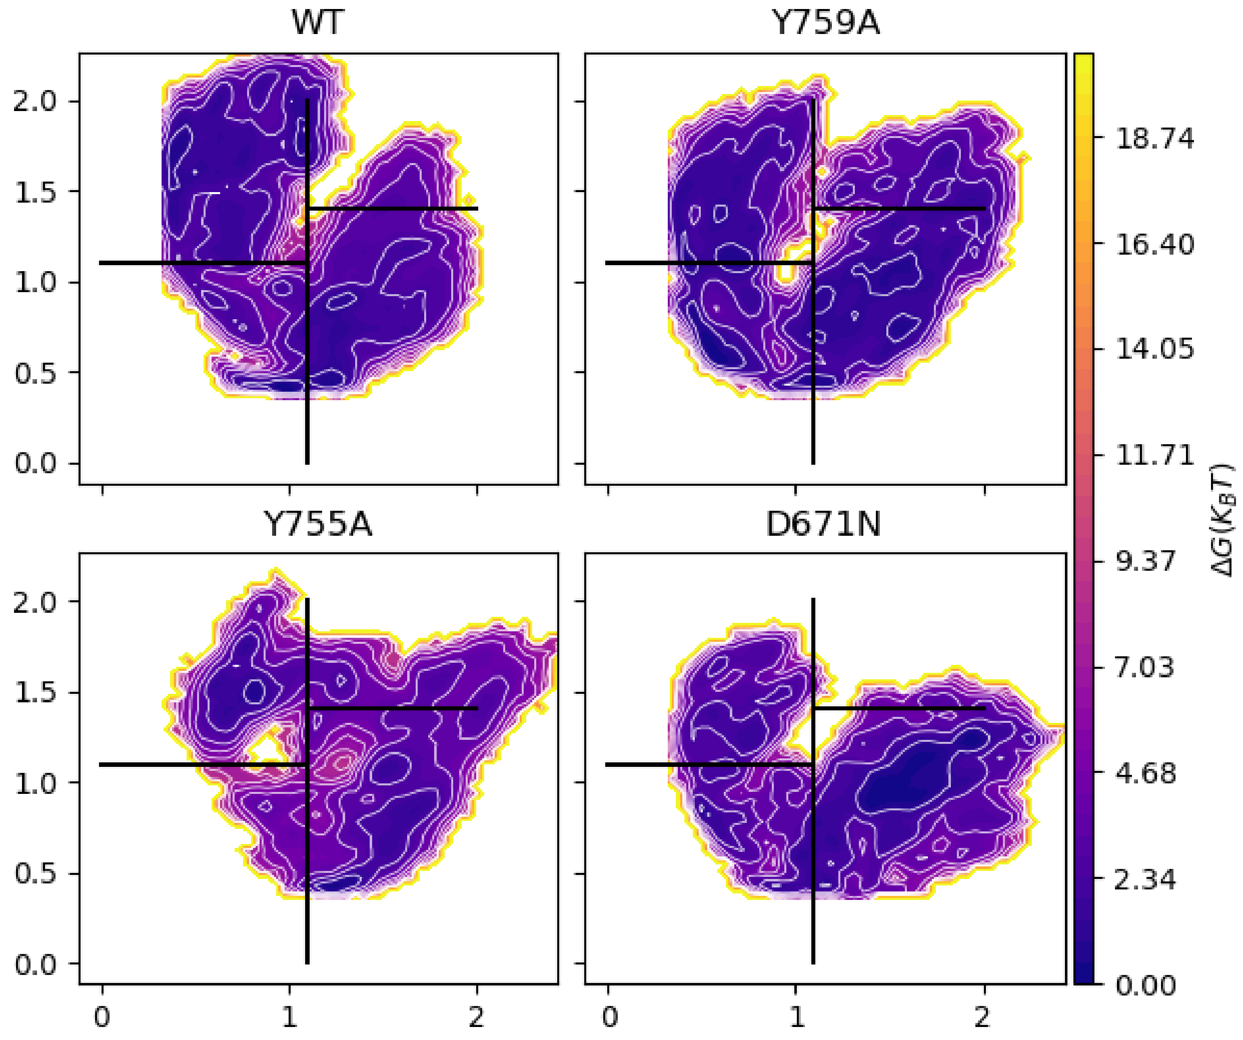


Figure 5: PMfs sampled for all four systems projected on Dunbrack co-ordinates, a) Wild type, b) D671N, c) Y755A and d) Y759A

## Using GrASP on our results

In Fig. 6 we show cryptic pocket predictions using GrASP[5] for various free energy minimum structures in DFG-in and DFG-out conformations for wild type DDR1. It is clear that we uncover new pockets by increasing sampling, and several of these correlate with druggable regions in other kinases, but further work must be done to investigate the usefulness of these pockets.

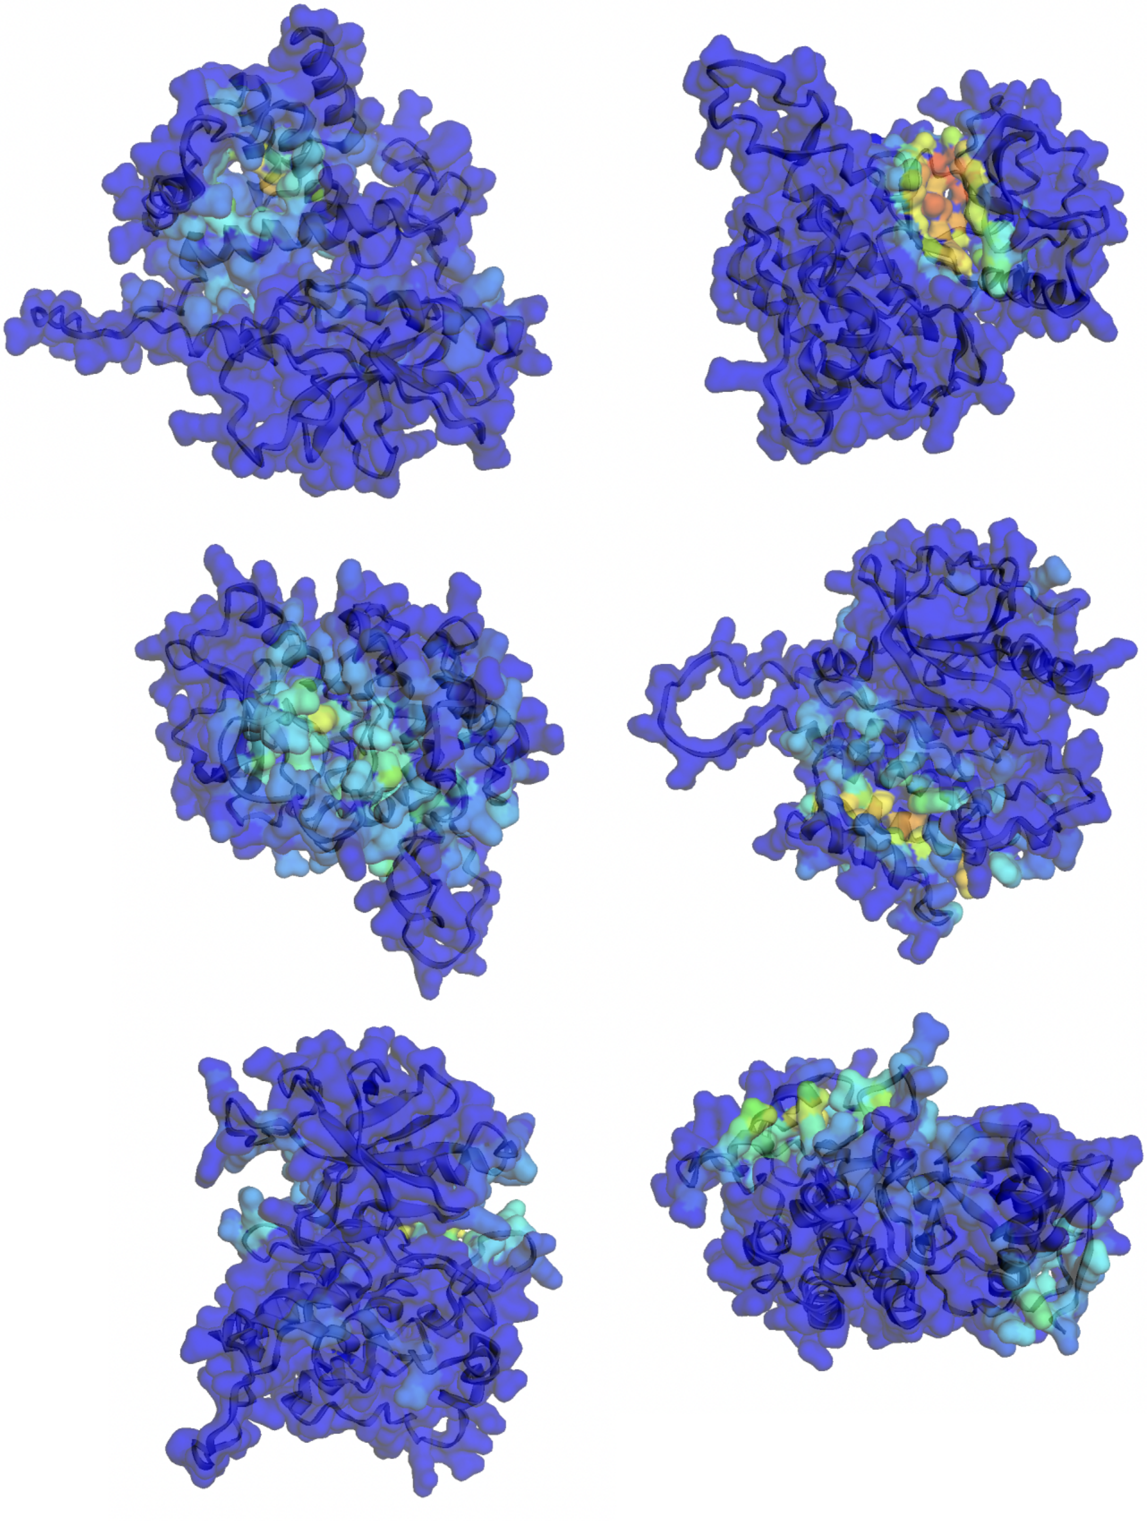

Figure 6: Cryptic pocket predictions for various free energy minimum structures in DFG-in and DFG-out conformations for wild type DDR1.

# References


(1) Narayan, B.; Fathizadeh, A.; Templeton, C.; He, P.; Arasteh, S.; Elber, R.; Buchete, N.-V.; Levy, R. M. The transition between active and inactive conformations of Abl kinase studied by rock climbing and Milestoning. *Biochimica et Biophysica Acta (BBA) - General Subjects* **2020**, *1864*, 129508.

(2) Modi, V.; Dunbrack, R. L. Defining a new nomenclature for the structures of active and inactive kinases. *Proceedings of the National Academy of Sciences* **2019**, *116*, 6818–6827.

(3) Meng, Y.; lin Lin, Y.; Roux, B. Computational Study of the "DFG-Flip" Conformational Transition in c-Abl and c-Src Tyrosine Kinases. *The Journal of Physical Chemistry B* **2015**, *119*, 1443–1456.

(4) da Silva, G. M.; Cui, J. Y.; Dalgarno, D. C.; Lisi, G. P.; Rubenstein, B. M. Predicting Relative Populations of Protein Conformations without a Physics Engine Using AlphaFold2. **2023**,

(5) Smith, Z.; Strobel, M.; Vani, B. P.; Tiwary, P. Graph Attention Site Prediction (GrASP): Identifying Druggable Binding Sites Using Graph Neural Networks with Attention. *bioRxiv* **2023**,
